# Supplementary material for: Simulating photonic devices with noisy optical elements
Source: arXiv:2311.10613 source file (2024-03-07)
Supplement: Supplementary file 1 [file circ_visualization.tex]

In this appendix we display the circuits that we implement for the simulations in Section \ref{tests}. The translations from circuit defined in Qiskit \cite{qiskit} to optical circuit are performed with the QiskitConverter functionality of Perceval \cite{Perceval}.
\begin{figure*}[htp]
\centering
\begin{minipage}{0.25\textwidth}
\includegraphics[width=\textwidth]{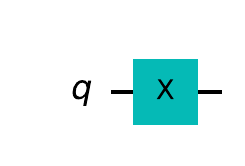}
\end{minipage}
\begin{minipage}{0.40\textwidth}
\includegraphics[width=\textwidth]{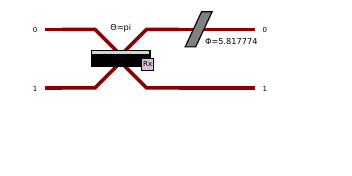}
\end{minipage}
\caption{On the left the circuit for the X gate in GBQC. On the right the corresponding optical circuit.}
\label{X_circuits}
\end{figure*}

\begin{figure*}[htp]
\centering
\begin{minipage}{0.25\textwidth}
\includegraphics[width=\textwidth]{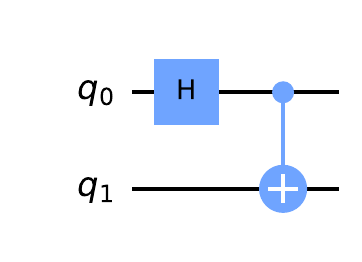}
\end{minipage}
\begin{minipage}{\textwidth}
\includegraphics[width=\textwidth]{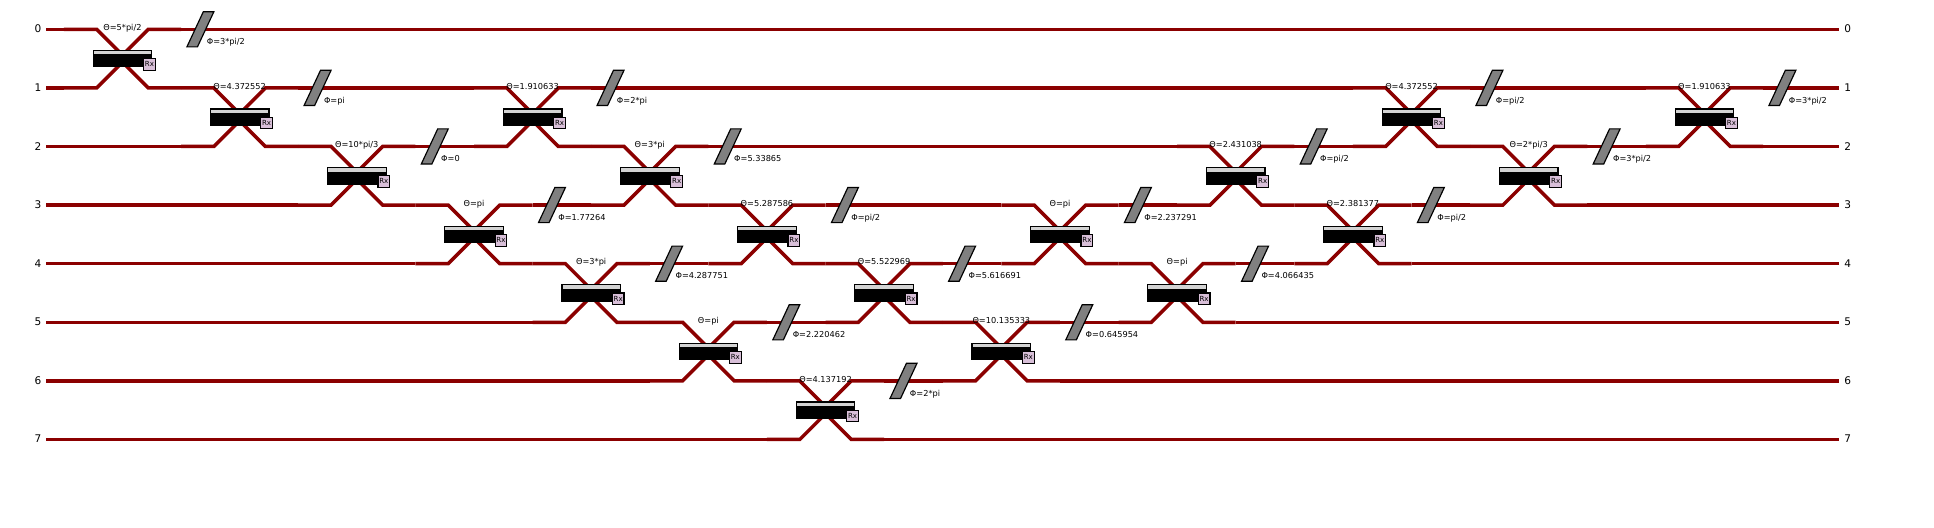}
\end{minipage}
\caption{On the top the circuit for the Bell state in GBQC. On the bottom the corresponding optical circuit.}
\label{Bell_circuits}
\end{figure*}

\begin{figure*}[htp]
\centering
\begin{minipage}{0.25\textwidth}
\includegraphics[width=\textwidth]{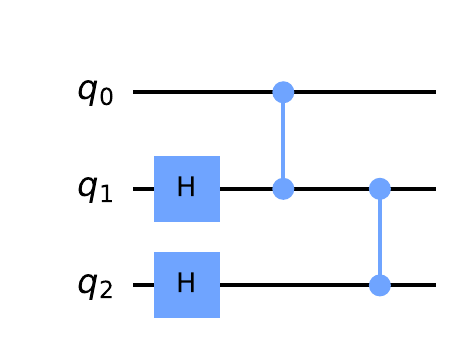}
\end{minipage}
\begin{minipage}{\textwidth}
\includegraphics[width=\textwidth]{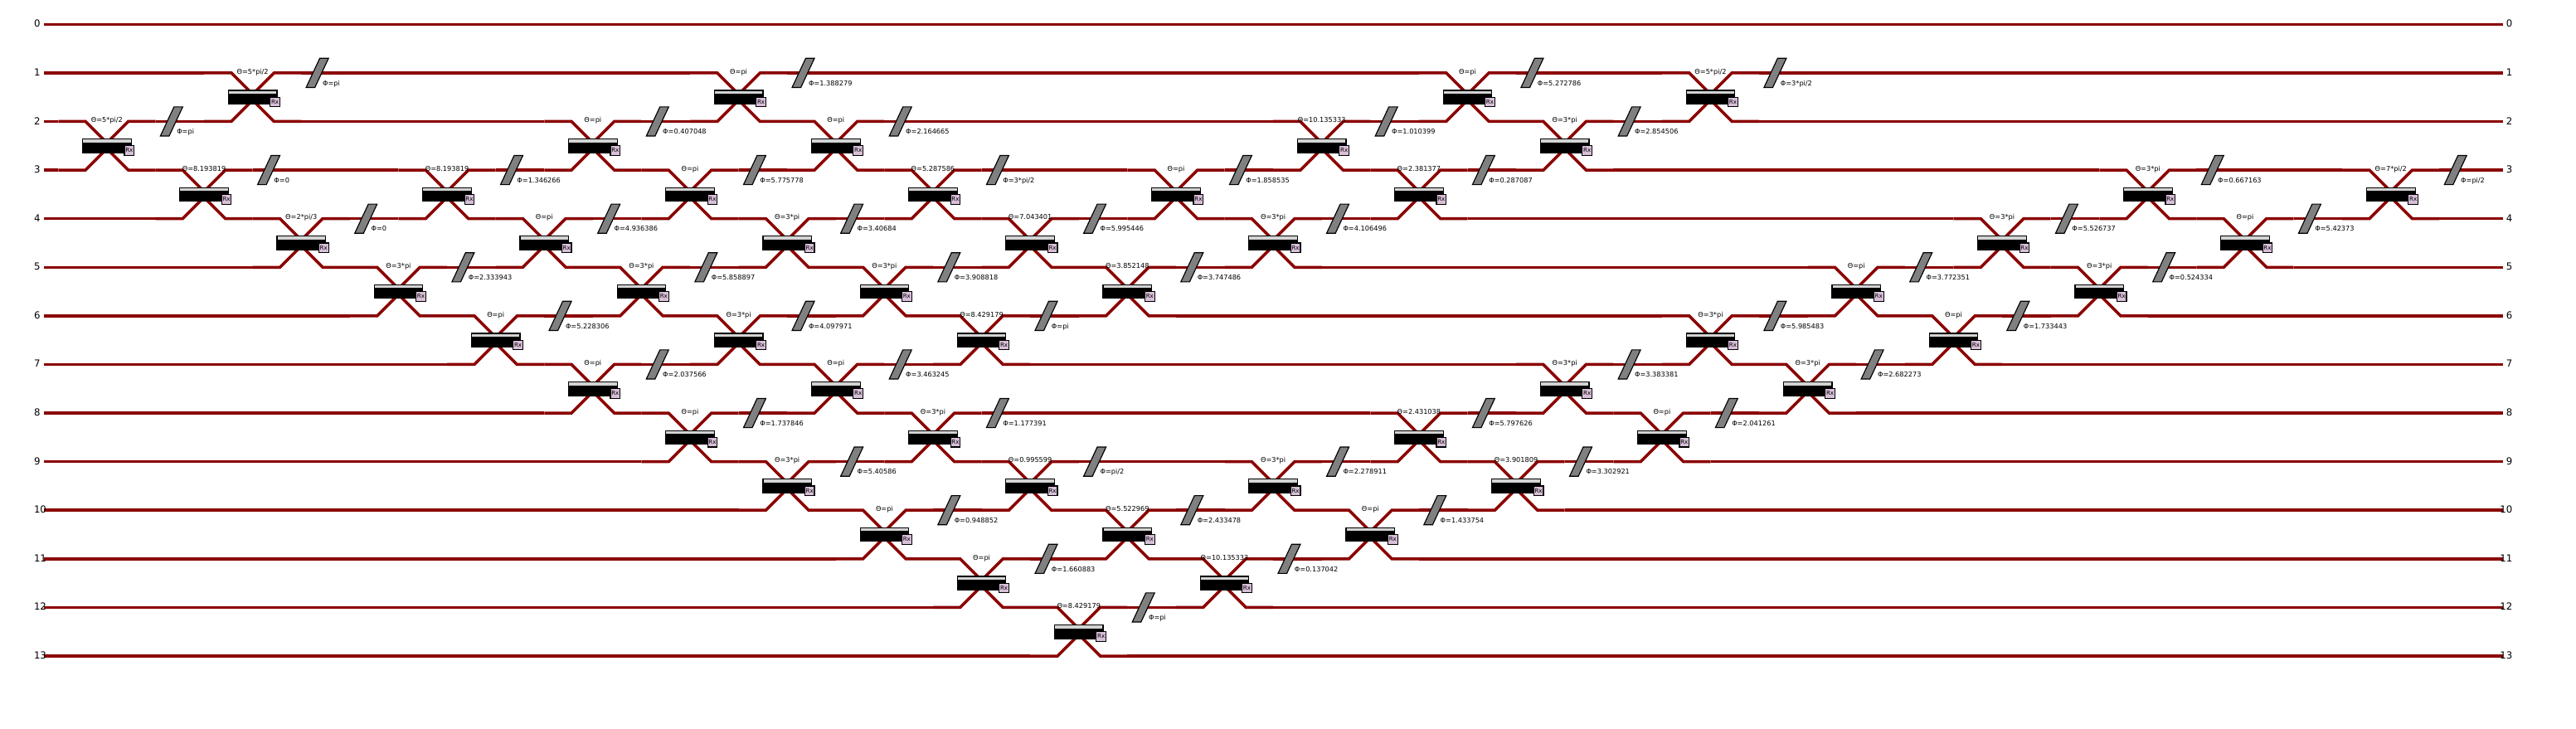}
\end{minipage}
\caption{On the top the circuit required to prepare the cluster state for the X gate in MBQC. On the bottom the corresponding optical circuit. Measurements for the MBQC are not shown.}
\label{MBQC_X_circuits}
\end{figure*}

\begin{figure*}[htp]
\centering
\begin{minipage}{\textwidth}
\includegraphics[width=\textwidth]{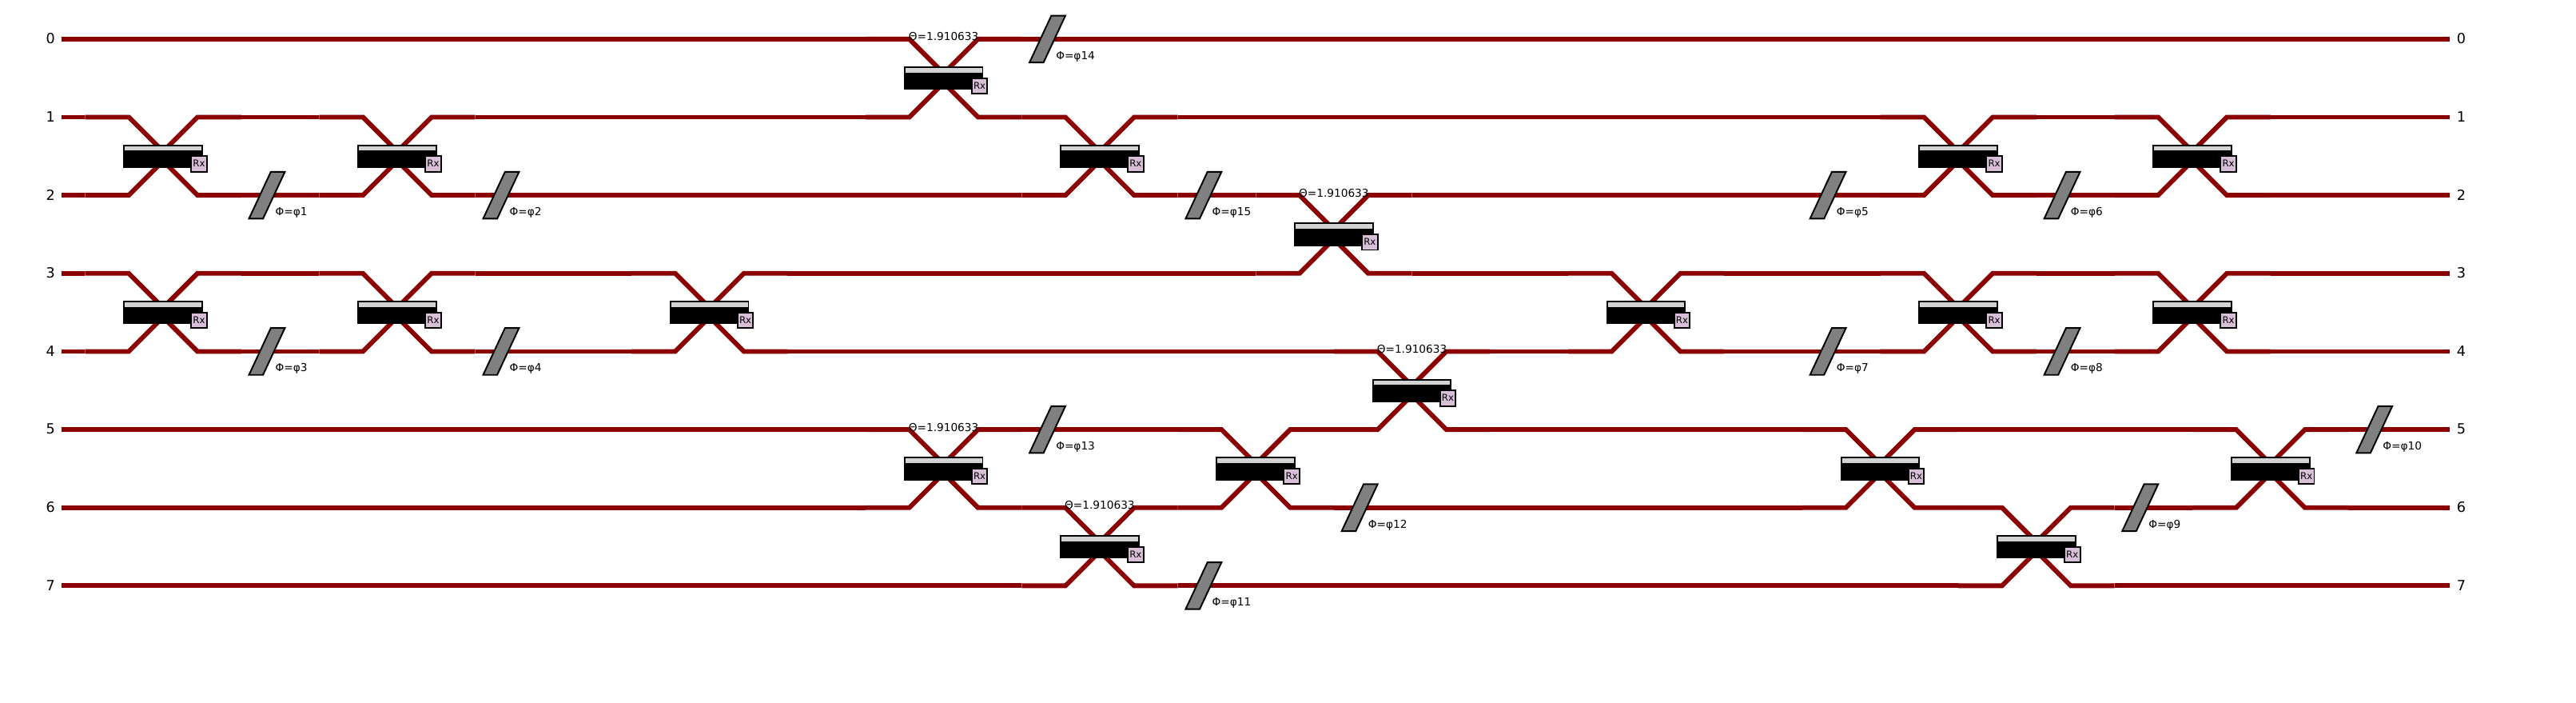}
\end{minipage}
\caption{Optical circuit ansatz for the VQA solving the max 2-cut on a square graph.}
\label{VQA_ansatz}
\end{figure*}
